# Supplementary material for: Canonical Correlation Analysis as Reduced Rank Regression in High Dimensions
Source: arXiv:2405.19539 source file (2026-09-03)
Supplement: Supplementary file 1 [file appendix_scalability.tex]

\subsection{Sparse Penalties in very large dimensions}

\subsection{Ridge Penalties in large dimensions}

Contrary to the $\ell_1$ case, ridge-penalty tend to shrink --- but not select variables. Consequently, the effective dimension of the problem does not shrink with the penalty. In many applications, particularly when working with fMRI data, we may encounter data with an extremely large number of features $p$. In this scenario, it is not possible to compute and store the inner product matrix $X^\top X  + \lambda K_x$ and, subsequently, find the corresponding $B_{\textit{OLS}}$ necessary for the CCA solution. We propose here a computational trick that allows us to avoid working with the inner product matrix, when the penalty matrix $K_X$ is easy to invert.

\begin{lemma}
To find the CCA solution in high dimension one can first compute the dual form of the OLS solution 
\begin{equation}
B_{\textit{OLS}} = K_X^{-1}X^\top(XK_X^{-1}X^\top+I)^{-1}\tilde Y
\label{eq:bols:alt}
\end{equation}
then find $\tilde V$ as the matrix containing the first $k$ eigenvectors of $\tilde Y ^T X B_{\textit{OLS}}.$
    
\end{lemma}

\begin{proof}
First we note that $B_{\textit{OLS}}$ is the solution to the normal equation  
$$X^\top X B_{\textit{OLS}} + \lambda K_XB_{\textit{OLS}} = X^\top \tilde Y.$$
Rearranging the terms gives
$$B_{\textit{OLS}} = K_X^{-1}X^\top (\tilde Y - X B_{\textit{OLS}}).$$
Denote residuals by $R = \tilde Y - X B_{\textit{OLS}}$, then 
$B_{\textit{OLS}} = K_X^{-1}X^\top R.$ Combining these two equations we obtain
$$R = \tilde Y - X K_X^{-1}X^\top R\quad\Longleftrightarrow\quad R = (X K_X^{-1}X^\top + I)^{-1}\tilde Y$$
yielding to (\ref{eq:bols:alt}).
\end{proof}

\xhdr{Computational cost}:  Note that we can pre-compute the ``hat'' matrix $H$, which requires:
    \begin{itemize}
        \item solving an equation $\tilde X = X K_X^{-1}$, which can be handled by sparse solvers (if the penalty matrix is sparse) or in parallel (if the penalty matrix is block-diagonal);
        \item finding $X\tilde X^\top$, which is $\mathcal O(n^2p)$;
        \item finding $X\tilde X^\top (X \tilde X^\top+I)^{-1}$, which is  $\mathcal O(n^3)$;
    \end{itemize}
Therefore, the cost of one iteration in the algorithm consists of:
\begin{itemize}
    \item $\mathcal O(q^3)$ for computing $(\Sigma_{YY}+K_Y)^{-\frac12}$;
    \item $O(nq^2)$ for computing $\tilde Y$;
    \item $O(n^2q+nq^2)$ for computing $\tilde Y_k$;
    \item $O(nq^2)$ for computing new values for imputation in $Y$.
\end{itemize}
